# Supplementary material for: Treatment of Herzberg-Teller and non-Condon effects in optical spectra with Hierarchical Equations of Motion
Source: arXiv:1807.07475 ancillary file (2018-07-19)
Supplement: Supplementary file 1 [file supplementary_material.pdf]

# Treatment of Herzberg-Teller and non-Condon effects in optical spectra with Hierarchical Equations of Motion: Supplementary Material

Joachim Seibt* and Tomáš Mančal

*Faculty of Mathematics and Physics, Ke Karlovu 5, 121 16 Prague 2, Czech Republic*

### Description of relaxation by using the standard Redfield approach in the framework of a vibronic basis representation in the time domain

To formulate the dissipative contribution to the Liouville-von-Neumann equation we choose the Redfield theory, as we assume the coupling between our electronic system and the thermodynamic bath to be weak. We define the following operator

$$\hat{\varLambda}_{el,mm,exc}(t) = \int_0^t d\tau C_{el}(\tau)(\hat{B}_m^\dagger \hat{B}_m)_{exc}(-\tau) \tag{SI 1}$$

with $\hat{B}_m^\dagger \hat{B}_m(-\tau) = \exp(i\hat{H}(-\tau))\hat{B}_m^\dagger \hat{B}_m \exp(-i\hat{H}(-\tau))$. Note that, different from the definition in [1], the upper integration border in Eq. (SI 1) is taken as variable. The dissipative contribution to the Liouville-von-Neumann equation can then be formulated as

$$\begin{aligned}\left(\frac{d\hat{\rho}}{dt}\right)_{diss,el} = &-\sum_m \Big[\hat{B}_m^\dagger \hat{B}_m, \hat{\varLambda}_{el,mm}(t)\hat{\rho}(t) \\ &-\hat{\rho}(t)\hat{\varLambda}^{(+)}_{el,mm}(t)\Big],\end{aligned} \tag{SI 2}$$

where the assumption of a variable upper integration border in $\hat{\varLambda}_{el,mm}(t)$ and its adjoint operator leads to a description of coherence decay on the same level as with the cumulant expansion technique from [2]. By representing $\hat{\rho}$, $\hat{K} = \sum_m \hat{B}_m^\dagger \hat{B}_m$ and $\hat{\varLambda}(t) = \sum_m \hat{\varLambda}_{el,mm}(t)$ in the vibronic basis, one can formulate the rate equation for population transfer in secular approximation as

$$\begin{aligned}\left(\frac{d\hat{\rho}}{dt}\right)_{ii} = &-\left(\sum_j \left(K_{ij}\varLambda_{ji}(t) + \varLambda^{(+)}_{ij}(t)K_{ji}\right)\right)\hat{\rho}_{ii}(t) \\ &+\sum_j \left(\varLambda_{ij}(t)K_{ji} + K_{ij}\varLambda^{(+)}_{ji}(t)\right)\hat{\rho}_{jj}(t).\end{aligned} \tag{SI 3}$$

* seibt@karlov.mff.cuni.cz

Transfer between the vibronic eigenstates leads to dephasing via life time broadening according to

$$\begin{aligned}\left(\frac{d\hat{\rho}}{dt}\right)_{ltb,ij} &= -\left(\sum_{j'} K_{ij'}\Lambda_{j'i}(t)\right)\hat{\rho}_{ij}(t)\\ &\quad -\left(\sum_{i'}\Lambda^{(+)}_{i'j}(t)K_{ji'}\right)\hat{\rho}_{ij}(t).\end{aligned} \tag{SI 4}$$

The corresponding contribution of pure dephasing is

$$\left(\frac{d\hat{\rho}}{dt}\right)_{pd,ij} = \Lambda_{ii}(t)K_{jj}\hat{\rho}_{ij}(t) + K_{ii}\Lambda^{(+)}_{jj}(t)\hat{\rho}_{ij}(t). \tag{SI 5}$$

**Derivation of Matsubara decomposition coefficients of an undamped oscillator entering in HEOM**

In analogy to the specification of the Feynman-Vernon functional (with general formulation in terms of correlation functions according to Eq. (36) from our article file) for the case of a Debye-Drude spectral density in Ref. [3], also undamped oscillator contributions can be treated. For the respective spectral density $J(\omega) = \frac{1}{2}S_{UO}\omega_{UO}\omega(\delta(\omega - \omega_{UO}) + \delta(\omega + \omega_{UO}))$ and under the assumption that the system components $\hat{V}^{\times}(\alpha,\alpha';t) = \hat{V}^{\times}(\alpha,\alpha') = \hat{V}(\alpha) - \hat{V}(\alpha')$ and $\hat{V}^{\circ}(\alpha,\alpha';t) = \hat{V}^{\circ}(\alpha,\alpha') = \hat{V}(\alpha) + \hat{V}(\alpha')$ of the system-bath interaction do not exhibit an explicit time-dependence, the Feynman-Vernon functional becomes

$$\begin{aligned}\mathcal{F}(\alpha,\alpha';t) = \exp\Bigg\{&-S_{UO}\omega_{UO}^2\int_0^t d\tau\left(\int_0^\tau d\tau'\hat{V}^{\times}(\alpha,\alpha')\times\left[\hat{V}^{\times}(\alpha,\alpha')\coth\left(\frac{\beta\omega_{UO}}{2}\right)\cos(\omega_{UO}(\tau-\tau'))\right.\right.\\ &\left.\left.-\,i\hat{V}^{\circ}(\alpha,\alpha')\sin(\omega_{UO}(\tau-\tau'))\right] + i\hat{V}^{\times}(\alpha,\alpha')\frac{1}{\omega_{UO}}\hat{V}^{\circ}(\alpha,\alpha')\right)\Bigg\}.\end{aligned} \tag{SI 6}$$

According to Fubini's theorem, this expression corresponds to

$$\begin{aligned}&\mathcal{F}(\alpha,\alpha';t)\\ &= \exp\Bigg\{-S_{UO}\omega_{UO}^2\left(\int_0^t d\tau'\int_{\tau'}^t d\tau\hat{V}^{\times}(\alpha,\alpha')\times\left[\hat{V}^{\times}(\alpha,\alpha')\coth\left(\frac{\beta\omega_{UO}}{2}\right)\cos(\omega_{UO}(\tau-\tau'))\right.\right.\\ &\quad\left.\left.-\,i\hat{V}^{\circ}(\alpha,\alpha')\sin(\omega_{UO}(\tau-\tau'))\right] + \int_0^t d\tau\hat{V}^{\times}(\alpha,\alpha')\frac{i}{\omega_{UO}}\hat{V}^{\circ}(\alpha,\alpha')\right)\Bigg\}\\ &= \exp\Bigg\{-S_{UO}\omega_{UO}^2\int_0^t d\tau'\hat{V}^{\times}(\alpha,\alpha')\times\left[\hat{V}^{\times}(\alpha,\alpha')\coth\left(\frac{\beta\omega_{UO}}{2}\right)\frac{\sin(\omega_{UO}(t-\tau'))-\sin(\omega_{UO}(\tau'-\tau'))}{\omega_{UO}}\right.\\ &\left.-i\hat{V}^{\circ}(\alpha,\alpha')\frac{-\cos(\omega_{UO}(t-\tau'))+\cos(\omega_{UO}(\tau'-\tau'))}{\omega_{UO}}\right] + \int_0^t d\tau\hat{V}^{\times}(\alpha,\alpha')\frac{i}{\omega_{UO}}\hat{V}^{\circ}(\alpha,\alpha')\Bigg\}\\ &= \exp\Bigg\{-S_{UO}\omega_{UO}^2\int_0^t d\tau'\hat{V}^{\times}(\alpha,\alpha')\times\left[\hat{V}^{\times}(\alpha,\alpha')\coth\left(\frac{\beta\omega_{UO}}{2}\right)\frac{\sin(\omega_{UO}(t-\tau'))}{\omega_{UO}}\right.\\ &\left.+i\hat{V}^{\circ}(\alpha,\alpha')\frac{\cos(\omega_{UO}(t-\tau'))}{\omega_{UO}}\right]\Bigg\}.\end{aligned} \tag{SI 7}$$

Taking the time-derivative of this expression, one obtains

$$\begin{aligned}
&\frac{\partial}{\partial t}\mathcal{F}(\alpha,\alpha';t)\\
&= \hat{V}^{\times}(\alpha,\alpha') \times \left[ -S_{UO}\omega_{UO}^2 \frac{\partial}{\partial t}\int_0^t d\tau' \left\{ \hat{V}^{\times}(\alpha,\alpha')\coth\left(\frac{\beta\omega_{UO}}{2}\right)\frac{\sin(\omega_{UO}(t-\tau'))}{\omega_{UO}} \right.\right.\\
&\left.\left. +i\hat{V}^{\circ}(\alpha,\alpha')\frac{\cos(\omega_{UO}(t-\tau'))}{\omega_{UO}} \right\}\right] \mathcal{F}(\alpha,\alpha';t)\\
&= -i\hat{V}^{\times}(\alpha,\alpha') \times \left[ -iS_{UO}\omega_{UO}^2 \left( \frac{i}{\omega_{UO}}\hat{V}^{\circ}(\alpha,\alpha') \right.\right.\\
&\left.\left. +\int_0^t d\tau' \left\{ \hat{V}^{\times}(\alpha,\alpha')\coth\left(\frac{\beta\omega_{UO}}{2}\right)\cos(\omega_{UO}(t-\tau')) - i\hat{V}^{\circ}(\alpha,\alpha')\sin(\omega_{UO}(t-\tau')) \right\} \right) \right] \mathcal{F}(\alpha,\alpha';t)\\
&= -i\hat{V}^{\times}(\alpha,\alpha') \times \left[ -iS_{UO}\omega_{UO}^2 \left( \frac{i}{\omega_{UO}}\hat{V}^{\circ}(\alpha,\alpha') \right.\right.\\
&+\int_0^t d\tau' \left\{ \hat{V}^{\times}(\alpha,\alpha')\coth\left(\frac{\beta\omega_{UO}}{2}\right)\frac{1}{2}\left(\exp(i\omega_{UO}(t-\tau')) + \exp(-i\omega_{UO}(t-\tau'))\right) \right.\\
&\left.\left.\left. -i\hat{V}^{\circ}(\alpha,\alpha')\frac{1}{2i}\left(\exp(i\omega_{UO}(t-\tau')) - \exp(-i\omega_{UO}(t-\tau'))\right) \right\} \right) \right] \mathcal{F}(\alpha,\alpha';t)\\
&= -i\hat{V}^{\times}(\alpha,\alpha') \times \left[ -iS_{UO}\omega_{UO}^2 \left( \frac{i}{\omega_{UO}}\hat{V}^{\circ}(\alpha,\alpha') \right.\right.\\
&+\int_0^t d\tau' \left\{ \exp(i\omega_{UO}(t-\tau'))\frac{1}{2}\left( \hat{V}^{\times}(\alpha,\alpha')\coth\left(\frac{\beta\omega_{UO}}{2}\right) - \hat{V}^{\circ}(\alpha,\alpha') \right) \right\}\\
&\left.\left. +\int_0^t d\tau' \left\{ \exp(-i\omega_{UO}(t-\tau'))\frac{1}{2}\left( \hat{V}^{\times}(\alpha,\alpha')\coth\left(\frac{\beta\omega_{UO}}{2}\right) + \hat{V}^{\circ}(\alpha,\alpha') \right) \right\} \right) \right] \mathcal{F}(\alpha,\alpha';t)\\
&= -\hat{\Phi}(\alpha,\alpha')\left( \hat{G}(\alpha,\alpha') + \int_0^t d\tau' \hat{\Xi}(\alpha,\alpha';\tau',t) \right)\mathcal{F}(\alpha,\alpha';t).
\end{aligned} \tag{SI 8}$$

The expression $\hat{G}(\alpha,\alpha') + \int_0^t d\tau' \hat{\Xi}(\alpha,\alpha';\tau',t)$ with $\hat{G}(\alpha,\alpha') = S_{UO}\omega_{UO}\hat{V}^{\circ}(\alpha,\alpha')$ can be combined with $\mathcal{F}(\alpha,\alpha';t)$ to yield $\mathcal{F}_1(\alpha,\alpha';t)$, which is multiplied with $-\hat{\Phi}(\alpha,\alpha') = -i\hat{V}^{\times}(\alpha,\alpha')$ in $\frac{\partial}{\partial t}\mathcal{F}(\alpha,\alpha';t)$. Taking the time-derivative of $\mathcal{F}_1(\alpha,\alpha';t)$, thereby identifying Matsubara decomposition frequencies $\gamma_{1,2} = \pm i\omega_{UO}$ and Matsubara decomposition coefficients

$$c_1 = \tilde{c}_2 = \frac{1}{2}S_{UO}\omega_{UO}^2\left(\coth\left(\frac{\beta\omega_{UO}}{2}\right) + 1\right), \tag{SI 9}$$

$$c_2 = \tilde{c}_1 = \frac{1}{2}S_{UO}\omega_{UO}^2\left(\coth\left(\frac{\beta\omega_{UO}}{2}\right) - 1\right) \tag{SI 10}$$

results in

$$\frac{\partial}{\partial t}\mathcal{F}_1 = -(\gamma_1+\gamma_2)\mathcal{F}_1 - i\left[(c_1+c_2)\hat{V}(\alpha) - (\tilde{c}_1+\tilde{c}_2)\hat{V}(\alpha')\right]\mathcal{F} - i\hat{V}^{\times}(\alpha,\alpha')\mathcal{F}_2 \tag{SI 11}$$

with $\mathcal{F}_2 = (\hat{G}(\alpha,\alpha') + \int_0^t d\tau' \hat{\Xi}(\alpha,\alpha';\tau',t))\mathcal{F}_1(\alpha,\alpha';t)$. The definition of coefficients and frequencies from the Matsubara decomposition leads to $\hat{\Xi}(\alpha,\alpha';\tau',t)) = \sum_k \exp(-\gamma_k(t-\tau))\hat{\Theta}_k(\alpha(\tau),\alpha'(\tau))$ with $\hat{\Theta}_k(\alpha(\tau),\alpha'(\tau)) = -i\left(c_k\hat{V}(\alpha(\tau)) - \tilde{c}_k\hat{V}(\alpha'(\tau))\right)$ (see Eq. (44), where an additional index $l$ for identification of the excited monomer appears).

**Calculation of effective Huang-Rhys factors**

To obtain a representation in the exciton basis, the appropriate transformation matrix is determined by diagonalization of the electronic part of the localized basis representation of the system Hamiltonian, which corresponds to Eq. (2) from the article without reorganization energy term. Basis transformation of the system-bath coupling components given in Eq. (4) from the article, thereby expressing them in terms of the displacements $d_m = \sqrt{\frac{2S_m}{\omega_m}}$ under the assumptions $\omega_1 = \omega_2 = \omega_0$, $S_{1,2} = \zeta_{1,2} S_D$ and $S_D = S_1 + S_2$, allows us to identify effective displacements and Huang-Rhys factors. Note that the system-bath coupling components, given in Eq. (4) from the article, are diagonal matrices with non-zero diagonal elements assigned to different basis states in the localized basis representation and can thus be treated like linearly independent vectors. In particular, they can be combined to yield orthonormal linear combinations associated with the redefined position coordinates $q_+ = \sqrt{\frac{1}{2}}(q_1 + q_2)$ and $q_- = \sqrt{\frac{1}{2}}(q_1 - q_2)$. By choosing this coordinate representation, which will turn out to be advantageous in the course of the further derivation, the effective displacements

$$d_{\alpha,+,0} = \sqrt{\frac{1}{2}}(\sqrt{\zeta_1}|\langle\alpha|1\rangle|^2 + \sqrt{\zeta_2}|\langle\alpha|2\rangle|^2)d_D \qquad \text{(SI 12)}$$

$$d_{\alpha,-,0} = \sqrt{\frac{1}{2}}(\sqrt{\zeta_1}|\langle\alpha|1\rangle|^2 - \sqrt{\zeta_2}|\langle\alpha|2\rangle|^2)d_D \qquad \text{(SI 13)}$$

are obtained, where Eqs. (SI 12) and (SI 13) are related to $q_+$ and $q_-$, respectively. In analogy to Eqs. (SI 12) and (SI 13) the effective Huang-Rhys factors can be defined as

$$S_{\alpha,+,0} = \frac{1}{2}(\sqrt{\zeta_1}|\langle\alpha|1\rangle|^2 + \sqrt{\zeta_2}|\langle\alpha|2\rangle|^2)^2 S_D \qquad \text{(SI 14)}$$

$$S_{\alpha,-,0} = \frac{1}{2}(\sqrt{\zeta_1}|\langle\alpha|1\rangle|^2 - \sqrt{\zeta_2}|\langle\alpha|2\rangle|^2)^2 S_D. \qquad \text{(SI 15)}$$

Because of the property of the contributions associated with $q_+$ and $q_-$ to be orthonormal, the effective Huang-Rhys factor of state $\alpha$ can be identified as $S_\alpha = S_{\alpha,+,0} + S_{\alpha,-,0}$, i.e. as the sum of contributions with involvement of squared displacements $d_{\alpha,+,0}$ and $d_{\alpha,-,0}$, but without any terms containing mixed products of them.

After basis transformation of the first-order Herzberg-Teller coupling contribution given in Eq. (5) from the article, the diagonal element assigned to state $\alpha$ can be identified as $H_{J^{(1)},\alpha\alpha} = \sum_l \sum_{m\neq l} J^{(1)}_{lm} \langle\alpha|l\rangle\langle m|\alpha\rangle \sqrt{2}\sqrt{\frac{1}{2}}(q_1 + q_2)$. To introduce an effective displacement with respect to $q_+$ under the influence of $J^{(1)}_{12}$, the contribution of $H_{J^{(1)},\alpha\alpha}$ to this effective displacement is determined via the assignment $H_{J^{(1)},\alpha\alpha} = d_{\alpha,+,J^{(1)}} \omega_0^2 \sqrt{\frac{1}{2}}(q_1 + q_2)$, which leads to $d_{\alpha,+,J^{(1)}} =$

$\frac{\sqrt{2}\sum_l \sum_{m\neq l} J^{(1)}_{lm}\langle\alpha|l\rangle\langle m|\alpha\rangle}{\omega_0^2}$. Furthermore, by introducing $\tilde{J}^{(1)}_{12} = \frac{J^{(1)}_{12}}{\sqrt{2}\omega_0}$ and by expressing $d_{\alpha,+,eff,J^{(1)}} = d_{\alpha,+,0} + d_{\alpha,+,J^{(1)}}$ in terms of Huang-Rhys factors, one arrives at

$$S_{\alpha,eff,J^{(1)}} = \frac{1}{2}\left(\sqrt{S_D}(\sqrt{\zeta_1}|\langle\alpha|1\rangle|^2 + \sqrt{\zeta_2}|\langle\alpha|2\rangle|^2) + \frac{2\sum_l \sum_{m\neq l} \tilde{J}^{(1)}_{lm}\langle\alpha|l\rangle\langle m|\alpha\rangle}{\omega_0}\right)^2 + \frac{1}{2}S_D(\sqrt{\zeta_1}|\langle\alpha|1\rangle|^2 - \sqrt{\zeta_2}|\langle\alpha|2\rangle|^2)^2. \tag{SI 16}$$

In the case of the second-order Herzberg-Teller coupling contribution from Eq. (6) from our article the appearance of products of position coordinates makes it more difficult to identify a corresponding displacement contribution. However, it is possible under the assumption that one of the position coordinates in each product term can be replaced by its average. For sufficiently strong excitonic coupling the average of the respective coordinate $q_k$ can be identified with its displacement in the excited state, which is scaled by an adjustable factor $f_k$ to account for increase of the displacement due to the influence of the coupling, so that the effective displacement becomes $f_k\sqrt{\zeta_k}d_D = f_k\sqrt{\zeta_k}\sqrt{\frac{2S_D}{\omega_0}}$ in the excited state. Under this assumption the contribution of the second-order Herzberg-Teller coupling term to the Huang-Rhys factor (without regarding the first-order term at the same time) can be obtained by taking analogous steps as in the corresponding derivation for the first-order term (here with rescaling of the Herzberg-Teller coupling constant as $\tilde{J}^{(2)}_{lm} = \frac{J^{(2)}_{lm}}{2\omega_0}$). The resulting effective Huang-Rhys factor is

$$S_{\alpha,eff,J^{(2)}} = \frac{1}{2}S_D\left((\sqrt{\zeta_1}|\langle\alpha|1\rangle|^2 + \sqrt{\zeta_2}|\langle\alpha|2\rangle|^2) + \frac{2(f_1\sqrt{\zeta_1} + f_2\sqrt{\zeta_2})\sum_l \sum_{m\neq l} \tilde{J}^{(2)}_{lm}\langle\alpha|l\rangle\langle m|\alpha\rangle}{\omega_0}\right)^2 + \frac{1}{2}S_D(\sqrt{\zeta_1}|\langle\alpha|1\rangle|^2 - \sqrt{\zeta_2}|\langle\alpha|2\rangle|^2)^2. \tag{SI 17}$$


[1] V. May and O. Kühn; *Charge and energy transfer dynamics in molecular systems*; Wiley-VCH, Weinheim (2011).

[2] S. Mukamel; *Principles of Nonlinear Optical Spectroscopy*; Oxford University Press, New York (1995).

[3] Y. Tanimura; J. Phys. Soc. Jpn. **75** 082001 (2006).
